# Supplementary material for: HiPerformer: Hierarchically Permutation-Equivariant Transformer for Time Series Forecasting
Source: arXiv:2305.08073 source file (2023-05-14)
Supplement: Supplementary file 1 [file 7_appendix.tex]

% \newpage
% \appendix
% \onecolumn
% \section{You \emph{can} have an appendix here.}

% You can have as much text here as you want. The main body must be at most $8$ pages long.
% For the final version, one more page can be added.
% If you want, you can use an appendix like this one, even using the one-column format.
